# Supplementary material for: Space-Aware Instruction Tuning: Dataset and Benchmark for Guide Dog Robots Assisting the Visually Impaired
Source: arXiv:2502.07183 source file (2025-02-12)
Supplement: Supplementary file 1 [file appendix.tex]

\section*{APPENDIX}
\section{Prompts}
\label{sec:app:prompts}

\subsection{System Prompts}
The same system prompts are used for both the baseline and the proposed pipeline. 
This prompt is used for generating responses for the destination, left, right, and path.

\begin{tcolorbox}[
colback=blue!10!white, 
colframe=blue!50!black, 
rounded corners, 
boxrule=0.5mm, 
title=System prompt for general response,
width=\columnwidth]
A chat between a human and an AI that understands visuals in English. In images, [x, y] denotes points: top-left [0.0, 0.0], bottom-right [1.0, 1.0]. Increasing x moves right; y moves down. Decreasing x moves left; y moves up. Bounding box: [x1, y1, x2, y2]. Image size: 1.0x1.0. The input image depicts the view from a pedestrian's position, taken at a point 80cm above the ground for pedestrian navigation purposes. The user is looking at the center [0.5, 0.5] of the image. Consider the starting point as the ground where the user is standing. Explain as if you were a navigation assistant explaining to a visually impaired person. Rules: 

1. Do not talk about detailed image coordinates. Never use pixel positional information. 2. Consider perspective view of the 2D image property.
\end{tcolorbox}

The following prompt was used to generate the response for the recommendation. Four additional rules were added to the previous prompt.

\begin{tcolorbox}[
colback=blue!10!white, 
colframe=blue!50!black, 
rounded corners, 
boxrule=0.5mm, 
title=System prompt for recommendation response,
width=\columnwidth]
A chat between a human and an AI that understands visuals in English. In images, [x, y] denotes points: top-left [0.0, 0.0], bottom-right [1.0, 1.0]. Increasing x moves right; y moves down. Decreasing x moves left; y moves up. Bounding box: [x1, y1, x2, y2]. Image size: 1.0x1.0. The input image depicts the view from a pedestrian's position, taken at a point 80cm above the ground for pedestrian navigation purposes. The user is looking at the center [0.5, 0.5] of the image. Consider the starting point as the ground where the user is standing. Explain as if you were a navigation assistant explaining to a visually impaired person. Rules: 

1. Do not talk about detailed image coordinates. Never use pixel positional information. 2. Consider perspective view of the 2D image property. 3. If the user is in front of a crosswalk, look for the pedestrian traffic light and tell me the color of the light. If there is a red pedestrian traffic light, say 'Stop and wait' option. 4. If there is an obstacle in the path obstructing the user's walk, say 'Stop and wait' option. 5. If the path leads the user into dangerous areas like roads or construction sites, say 'Stop and wait' option. 6. If the path is clear of obstacles, say 'Follow the path' option. 
\end{tcolorbox}

If the object information is added to the prompt, below prompt is added at the end of the system prompt. In the below example, we assume the two objects are detected, a truck at [0.2493, 0.2294, 1.0, 0.6915], a car at [0.0001, 0.4229, 0.1183, 0.5134] and a bollard at [0.1272, 0.5514, 0.1618, 0.7771].

\begin{tcolorbox}[
colback=blue!10!white, 
colframe=blue!50!black, 
rounded corners, 
boxrule=0.5mm, 
title=System prompt for recommendation response,
width=\columnwidth]
The image contains objects, truck [0.2493, 0.2294, 1.0, 0.6915], car [0.0001, 0.4229, 0.1183, 0.5134], bollard [0.1272, 0.5514, 0.1618, 0.7771].

\end{tcolorbox}

\subsection{User Prompts for Region-Prompt Method}
The four prompts below are used for the baseline system. All information about the destination and path is included in the prompt. In the following example, we assume the destination is at [0.5079, 0.502].

\begin{tcolorbox}[
colback=red!10!white, 
colframe=red!50!black, 
rounded corners, 
boxrule=0.5mm, 
title=User prompt for destination description,
width=\columnwidth]
Assume the user's destination is the point [0.5079, 0.502] in the image. Provide a one-sentence description of the destination where the user's path is heading. Example 1) The destination is ahead on the sidewalk. Example 2) The destination is ahead on the car road. Example 3) The destination is ahead but is obscured by a truck. Example 4) The destination is ahead at the entrance of the building. 
\end{tcolorbox}

\begin{tcolorbox}[
colback=red!10!white, 
colframe=red!50!black, 
rounded corners, 
boxrule=0.5mm, 
title=User prompt for left description,
width=\columnwidth]
Assume the user is moving along a 2-meter-wide path from the starting point [0.5, 1.0] to the destination point [0.5079, 0.502] in the image. Analyze the input image and provide a one-sentence description that includes what is located closely to the left of the path. If there are no special objects other than the floor, say 'nothing'. Example 1) There are cars on the left side. Example 2) There are nothing than the floor on the left side.
\end{tcolorbox}

\begin{tcolorbox}[
colback=red!10!white, 
colframe=red!50!black, 
rounded corners, 
boxrule=0.5mm, 
title=User prompt for right description,
width=\columnwidth]
Assume the user is moving along a 2-meter-wide path from the starting point [0.5, 1.0] to the destination point [0.5079, 0.502] in the image. Analyze the input image and provide a one-sentence description that includes what is located closely to the right of the path. If there are no special objects other than the floor, say 'nothing'. Example 1) There are people on the right side. Example 2) There are nothing than the floor on the right side. 
\end{tcolorbox}

\begin{tcolorbox}[
colback=red!10!white, 
colframe=red!50!black, 
rounded corners, 
boxrule=0.5mm, 
title=User prompt for path description,
width=\columnwidth]
Assume the user is moving along a 2-meter-wide path from the starting point [0.5, 1.0] to the destination point [0.5079, 0.502] in the image. Analyze the input image and provide a one-sentence description of what objects are on the path. Example 1) There are cars and people on the path. Example 2) There are nothing on the path. 
\end{tcolorbox}

\subsection{User Prompts for Masked-Image Method}

\begin{tcolorbox}[
colback=green!10!white, 
colframe=green!50!black, 
rounded corners, 
boxrule=0.5mm, 
title=User prompt for destination description,
width=\columnwidth]
Assume the visible area in the image is the user's path and the user moves forward along the visible area of the image. Provide a one-sentence description of the destination where the user's path is heading. Example 1) The destination is ahead on the sidewalk. Example 2) The destination is ahead on the car road. Example 3) The destination is ahead but is obscured by a truck. Example 4) The destination is ahead at the entrance of the building. 
\end{tcolorbox}

\begin{tcolorbox}[
colback=green!10!white, 
colframe=green!50!black, 
rounded corners, 
boxrule=0.5mm, 
title=User prompt for left description,
width=\columnwidth]
Assume the visible area in the image is to the left of the user's path. Analyze the visible area and provide a one-sentence description that includes what is located closely to the left of the path. If there are no special objects other than the floor, say 'nothing'. Example 1) There are cars on the left side. Example 2) There are nothing than the floor on the left side. 
\end{tcolorbox}

\begin{tcolorbox}[
colback=green!10!white, 
colframe=green!50!black, 
rounded corners, 
boxrule=0.5mm, 
title=User prompt for right description,
width=\columnwidth]
Assume the visible area in the image is to the right of the user's path. Analyze the visible area and provide a one-sentence description that includes what is located closely to the right of the path. If there are no special objects other than the floor, say 'nothing'. Example 1) There are people on the right side. Example 2) There are nothing than the floor on the right side. 
\end{tcolorbox}

\begin{tcolorbox}[
colback=green!10!white, 
colframe=green!50!black, 
rounded corners, 
boxrule=0.5mm, 
title=User prompt for path description,
width=\columnwidth]
Assume the visible area in the image is the user's path and the user moves forward along the visible area of the image. Analyze the visible area and provide a one-sentence description of what objects are on the path. Example 1) There are cars and people on the path. Example 2) There are nothing on the path. 
\end{tcolorbox}

\subsection{User Prompts for Both Region-Prompt and Masked-Image Methods}

\begin{tcolorbox}[
colback=orange!10!white, 
colframe=orange!50!black, 
rounded corners, 
boxrule=0.5mm, 
title=User prompt for whole image description,
width=\columnwidth]
Describe where the user is located based on the image. If the user is in front of a crosswalk, look for the pedestrian traffic light and tell me the color of the light. Example 1) The user is in front of a crosswalk. The pedestrian traffic light is red. Example 2) The user is in front of a construction site. 
\end{tcolorbox}

\begin{tcolorbox}[
colback=orange!10!white, 
colframe=orange!50!black, 
rounded corners, 
boxrule=0.5mm, 
title=User prompt for recommendation,
width=\columnwidth]
% The image description is following: \textit{The destination is ahead on the car road, but it is partially obscured by a green garbage truck.  There is a curb on the left side of the path.  There is a green garbage truck parked on the right side of the path.  There is a large green trash truck on the path.  The user is in front of a crosswalk. There is a pedestrian traffic light visible in the image, and it is displaying a red signal.} Based on the current description, evaluate the user is able to move along the path without collision or collide with other objects. Then, select the most appropriate action: 'Follow the path' or 'Stop and wait'. Say only the answer, explaining the selection and the reason in two sentences.  Example 1) Stop and wait. A car is on the path, so walking to the destination is impossible.  Example 2) Follow the path. The path is clear of obstacles, so walking to the destination is possible.  Example 3) Stop and wait. It is in front of the crosswalk and the pedestrian traffic light is red, so walking to the destination is impossible.  Say only the answers. 
The image description is following: \textit{\{Concatenated-Five-Descriptions\}} Based on the current description, evaluate the user is able to move along the path without collision or collide with other objects. Then, select the most appropriate action: 'Follow the path' or 'Stop and wait'. Say only the answer, explaining the selection and the reason in two sentences.  Example 1) Stop and wait. A car is on the path, so walking to the destination is impossible.  Example 2) Follow the path. The path is clear of obstacles, so walking to the destination is possible.  Example 3) Stop and wait. It is in front of the crosswalk and the pedestrian traffic light is red, so walking to the destination is impossible.  Say only the answers. 
\end{tcolorbox}

\subsection{System and User Prompts for LLM Judge}
\begin{tcolorbox}[
colback=yellow!10!white, 
colframe=yellow!50!black, 
rounded corners, 
boxrule=0.5mm, 
title=System prompt for LLM Judge,
width=\columnwidth]
Please act as an impartial judge and evaluate the quality of the description provided by an AI assistant to the user. Your evaluation should consider correctness and helpfulness. You will be given a reference description and the assistant's description. You evaluation should focus on the assistant's description. Begin your evaluation by comparing the assistant's description with the reference description. Identify and correct any mistakes. Be as objective as possible. After providing your explanation, you must rate the response on a scale of 1 to 10 by strictly following this format: "[[rating]]", for example: "Rating: [[5]]". 

\end{tcolorbox}

\begin{tcolorbox}[
colback=yellow!10!white, 
colframe=yellow!50!black, 
rounded corners, 
boxrule=0.5mm, 
title=User prompt for LLM Judge,
width=\columnwidth]
\textless|The Start of Reference Description|\textgreater \\
\textit{\{reference\_description\}} \\
\textless|The End of Reference Description|\textgreater \\

\medskip

\textless|The Start of Assistant A's Description|\textgreater \\
\textit{\{assistant\_description\}} \\
\textless|The End of Assistant A's Description|\textgreater
\end{tcolorbox}

\subsection{System and User Prompts of Single-turn Query}

\begin{tcolorbox}[
colback=cyan!10!white, 
colframe=cyan!50!black, 
rounded corners, 
boxrule=0.5mm, 
title=System prompt of single-turn query,
width=\columnwidth]
A chat between a human and an AI that understands visuals in English. In images, [x, y] denotes points: top-left [0.0, 0.0], bottom-right [1.0, 1.0]. Increasing x moves right; y moves down. Decreasing x moves left; y moves up. Bounding box: [x1, y1, x2, y2]. Image size: 1.0x1.0.The input image depicts the view from a pedestrian's position, taken at a point 80cm above the ground for pedestrian navigation purposes. The user is looking at the center [0.5, 0.5] of the image. Consider the starting point as the ground where the user is standing. Explain as if you were a navigation assistant explaining to a visually impaired person. Rules: 

1. Do not talk about detailed image coordinates. Never use pixel positional information. 2. Consider perspective view of the 2D image property. 3. If the user is in front of a crosswalk, look for the pedestrian traffic light and tell me the color of the light. If there is a red pedestrian traffic light, say 'Stop and wait' option. 4. If there is an obstacle in the path obstructing the user's walk, say 'Stop and wait' option. 5. If the path leads the user into dangerous areas like roads or construction sites, say 'Stop and wait' option. 6. If the path is clear of obstacles, say 'Follow the path' option. 
\end{tcolorbox}

\begin{tcolorbox}[
colback=cyan!10!white, 
colframe=cyan!50!black, 
rounded corners, 
boxrule=0.5mm, 
title=User prompt of single-turn query,
width=\columnwidth]
Assume the user is moving along a 2-meter-wide path from the starting point [0.5, 1.0] to the destination point [0.5079, 0.502] in the image. Provide the response in a structured format with numbered sections to separate the details clearly: 

1. Destination (x, y) Description: 

Provide a one-sentence description of the destination where the user's path is heading. Example 1) The destination is ahead on the sidewalk. Example 2) The destination is ahead on the car road. Example 3) The destination is ahead but is obscured by a truck. Example 4) The destination is ahead at the entrance of the building. 

2. Left Side of the Path: 

Analyze the input image and provide a one-sentence description that includes what is located closely to the left of the path. If there are no special objects other than the floor, say 'nothing'. Example 1) There are cars on the left side. Example 2) There are nothing than the floor on the left side. 

3. Right Side of the Path: 

Analyze the input image and provide a one-sentence description that includes what is located closely to the right of the path. If there are no special objects other than the floor, say 'nothing'. Example 1) There are people on the right side. Example 2) There are nothing than the floor on the right side. 

4. Path Description: 

Analyze the input image and provide a one-sentence description of what objects are on the path. Example 1) There are cars and people on the path. Example 2) There are nothing on the path. 

5. Overall Scene and Pedestrian Traffic Light: 

Describe where the user is located based on the image. If the user is in front of a crosswalk, look for the pedestrian traffic light and tell me the color of the light. Example 1) The user is in front of a crosswalk. The pedestrian traffic light is red. Example 2) The user is in front of a construction site. 

6. Walkability Evaluation: 

Based on the current description, evaluate the user is able to move along the path without collision or collide with other objects. Then, select the most appropriate action: 'Follow the path' or 'Stop and wait'. Say only the answer, explaining the selection and the reason in two sentences. Example 1) Stop and wait. A car is on the path, so walking to the destination is impossible. Example 2) Follow the path. The path is clear of obstacles, so walking to the destination is possible. Example 3) Stop and wait. It is in front of the crosswalk and the pedestrian traffic light is red, so walking to the destination is impossible. 

\end{tcolorbox}

\subsection{Ablation Study of Prompting with Detection Information}
Using a pedestrian-related object detector to explicitly include the class and locations of objects present in the image within the prompt can be helpful for VLMs, as it provides information that might otherwise be missed in the image. Table~\ref{table:det_info} shows the results of whether this method improves VLM image descriptions based on two metrics, the LLM Judge and BERT Score. According to the results, the LLM Judge metric indicates that omitting detection information leads to slightly more accurate descriptions than providing it. In contrast, the BERT Score consistently shows better performance when detection information is provided. In our study’s pipeline, we adopted the method of using detection information to generate the training dataset.

\begin{table}[!ht]
    \caption{Performance comparison based on LLM Judge and BERT Score metrics with and without detection information}
    \centering
    \begin{tabular}{|l|l|l|l|l|}
    \hline
        Method (Metric) & Dest & Left & Right & Path \\ \hhline{|=|=|=|=|=|}
%        w/ det info (LLM Judge)  & 4.35 & 3.20 & 3.09 & 2.45 \\ \hline
%        w/o info (LLM Judge)     & 4.40 & 3.19 & 3.15 & 2.61 \\ \hhline{|=|=|=|=|=|}
        w/ det info (LLM Judge)  & 4.49 & 3.04 & 2.84 & 2.28 \\ \hline
        w/o info (LLM Judge)     & 4.49 & 3.03 & \textbf{2.99} & \textbf{2.43} \\ \hhline{|=|=|=|=|=|}
        w/ det info (BERT Score) & \textbf{0.7398} & \textbf{0.7674} & \textbf{0.7637} & \textbf{0.6857} \\ \hline
        w/o info (BERT Score)    & 0.7372 & 0.7656 & 0.7609 & 0.6831 \\ \hline
    \end{tabular}
    \label{table:det_info}
\end{table}
